# Supplementary material for: FORML: A Riemannian Hessian-free Method for Meta-learning on Stiefel Manifolds
Source: arXiv:2402.18605 source file (2024-05-31)
Supplement: Supplementary file 1 [file Appendix.tex]

\section*{Appendix} \label{Appendix}
